# Supplementary material for: Inside the Visual Mind: Neuroscience-Motivated Concept Circuits for Interpreting and Steering Vision Transformers
Source: arXiv:2606.06664 source file (2026-06-04)
Supplement: Supplementary file 1 [file localization_additional.tex]

\begin{figure}[t]
  \centering
  \fbox{\rule{0pt}{1.0in} \rule{0.95\linewidth}{0pt}}
   % \includegraphics[width=1.0\linewidth]{img/localization.pdf}
   % \vspace{-15pt}
   \caption{
   Concept localization
   }
   % \vspace{-15pt}
   \label{fig:localization_additional}
\end{figure}
