# Supplementary material for: Inside the Visual Mind: Neuroscience-Motivated Concept Circuits for Interpreting and Steering Vision Transformers
Source: arXiv:2606.06664 source file (2026-06-04)
Supplement: Supplementary file 2 [file spurious_correlation_additional.tex]

% \begin{wrapfigure}{r}{0.6\textwidth}
% \vspace{-18pt}
\begin{figure}[ht]
    \centering
  % \begin{center}
  \fbox{\rule{0pt}{2.2in} \rule{0.95\linewidth}{0pt}}
  % \includegraphics[width=0.6\textwidth]{img/failure_mode.pdf}
  % \end{center}
  % \captionsetup{justification=raggedright, font=it}
  \vspace{-8pt}
  \caption{
  Qualitative examples of steering on WaterBird dataset.
  }
  \label{fig:spurious_correlation_additional}
\end{figure}

% \vspace{-15pt}
% \end{wrapfigure}
